# Supplementary material for: Analysis of Estimating the Bayes Rule for Gaussian Mixture Models with a Specified Missing-Data Mechanism
Source: arXiv:2210.13785 source file (2023-12-29)
Supplement: Supplementary file 1 [file Supplementary.pdf]

# Supplementary material for “Semi-supervised Learning: Estimating the Bayes Rule under a Specified Missing-Data Mechanism”

September 3, 2023

## Plot of ARE for two-class normal homoscedastic model

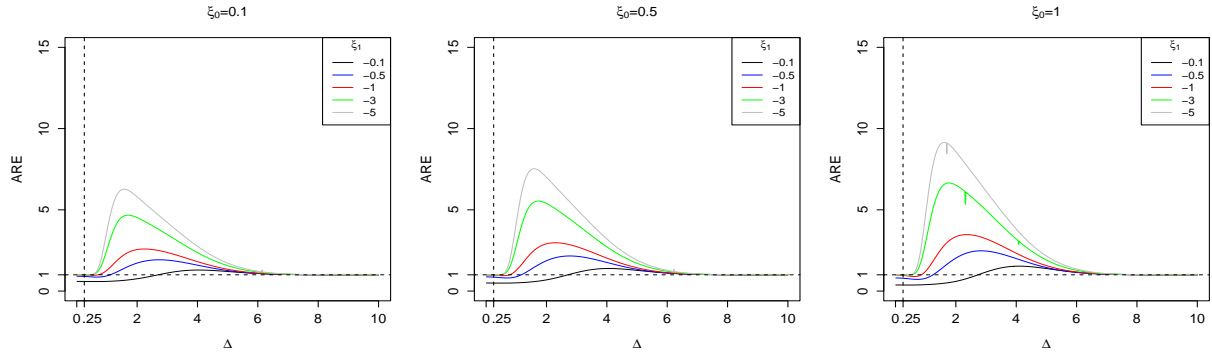

Figure 1: Plot of the asymptotic relative efficiency  $\text{ARE}(\boldsymbol{\beta}_{\text{PC}}^{(\text{full})}, \boldsymbol{\beta}_{\text{CC}})$  versus the squared root of the squared Mahalanobis distance between the two classes,  $\Delta$ , for  $\pi_1 = 0.1$ .

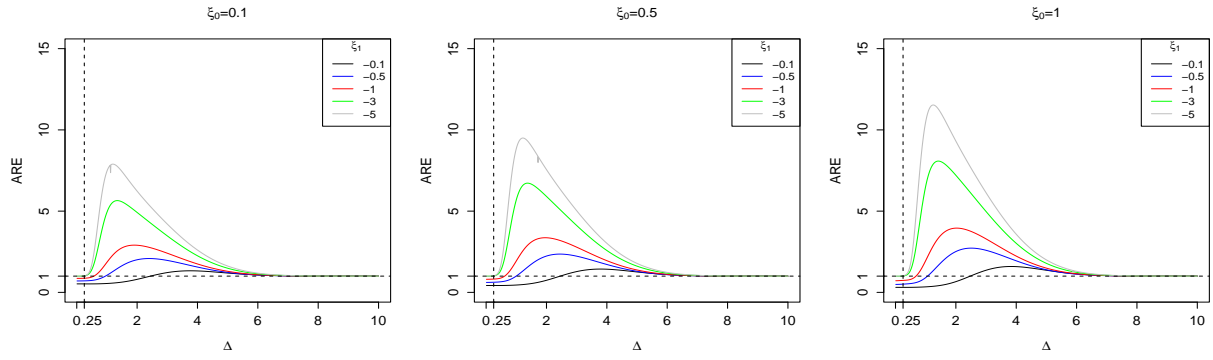

Figure 2: Plot of the asymptotic relative efficiency  $\text{ARE}(\boldsymbol{\beta}_{\text{PC}}^{(\text{full})}, \boldsymbol{\beta}_{\text{CC}})$  versus the squared root of the squared Mahalanobis distance between the two classes,  $\Delta$ , for  $\pi_1 = 0.2$ .

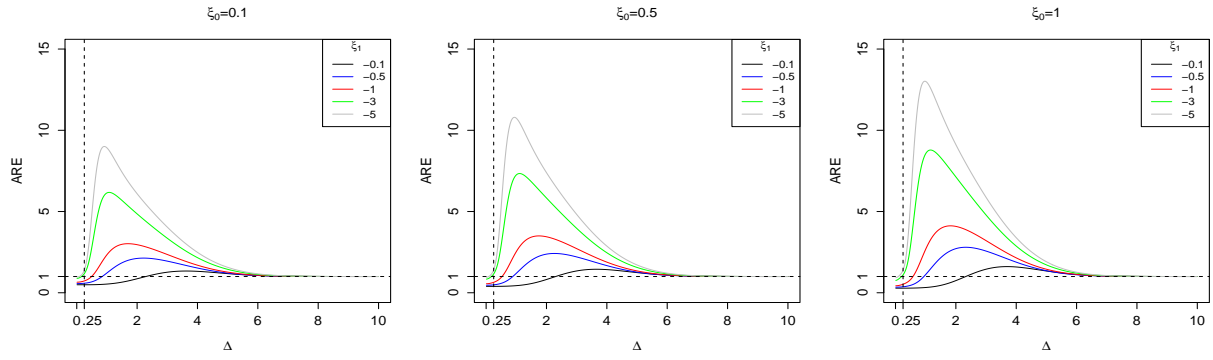

Figure 3: Plot of the asymptotic relative efficiency  $\text{ARE}(\boldsymbol{\beta}_{\text{PC}}^{(\text{full})}, \boldsymbol{\beta}_{\text{CC}})$  versus the squared root of the squared Mahalanobis distance between the two classes,  $\Delta$ , for  $\pi_1 = 0.3$ .

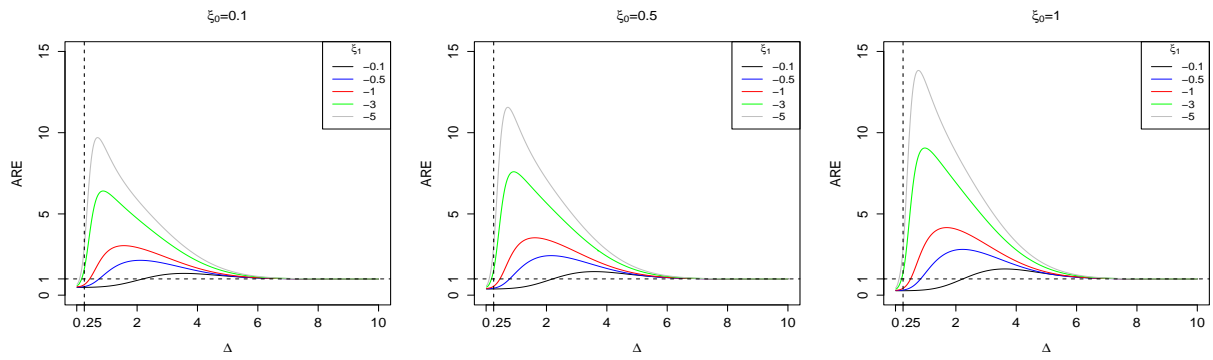

Figure 4: Plot of the asymptotic relative efficiency  $\text{ARE}(\boldsymbol{\beta}_{\text{PC}}^{(\text{full})}, \boldsymbol{\beta}_{\text{CC}})$  versus the squared root of the squared Mahalanobis distance between the two classes,  $\Delta$ , for  $\pi_1 = 0.4$ .

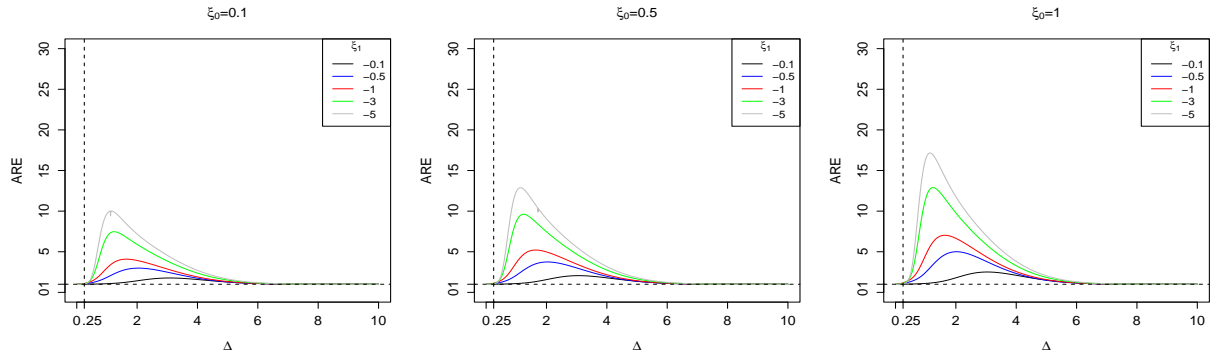

Figure 5: Plot of the asymptotic relative efficiency  $\text{ARE}(\boldsymbol{\beta}_{\text{PC}}^{(\text{full})}, \boldsymbol{\beta}_{\text{PC}}^{(\text{ig})})$  versus the squared root of the squared Mahalanobis distance between the two classes,  $\Delta$ , for  $\pi_1 = 0.1$ .

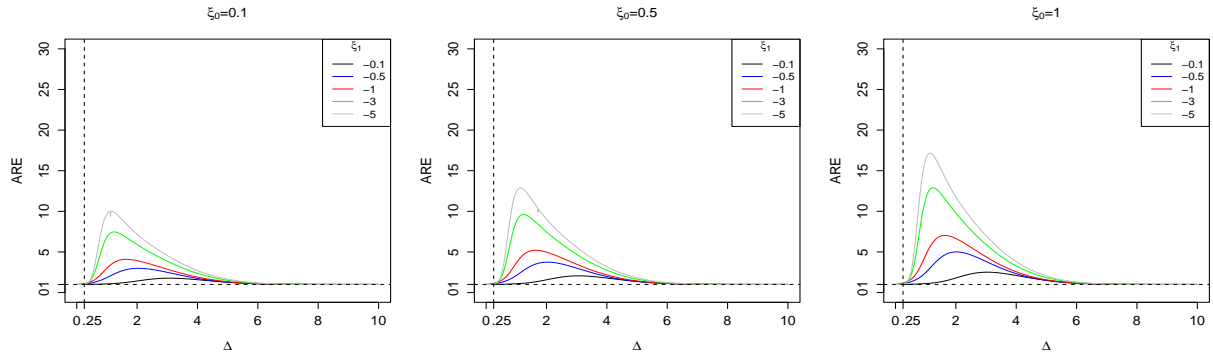

Figure 6: Plot of the asymptotic relative efficiency  $\text{ARE}(\boldsymbol{\beta}_{\text{PC}}^{(\text{full})}, \boldsymbol{\beta}_{\text{PC}}^{(\text{ig})})$  versus the squared root of the squared Mahalanobis distance between the two classes,  $\Delta$ , for  $\pi_1 = 0.2$ .

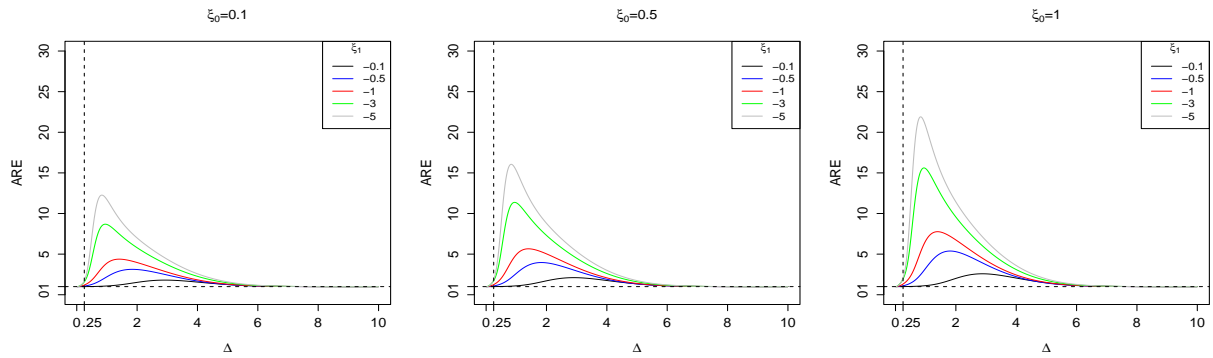

Figure 7: Plot of the asymptotic relative efficiency  $\text{ARE}(\boldsymbol{\beta}_{\text{PC}}^{(\text{full})}, \boldsymbol{\beta}_{\text{PC}}^{(\text{ig})})$  versus the squared root of the squared Mahalanobis distance between the two classes,  $\Delta$ , for  $\pi_1 = 0.3$ .

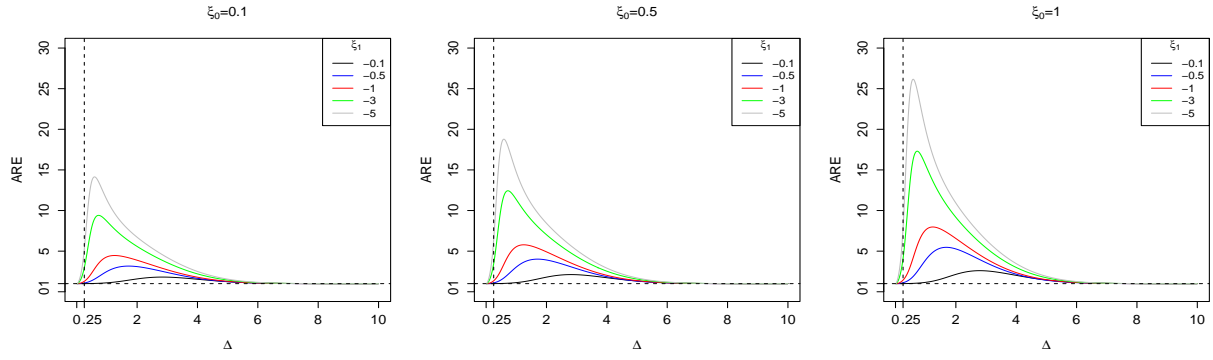

Figure 8: Plot of the asymptotic relative efficiency  $\text{ARE}(\boldsymbol{\beta}_{\text{PC}}^{(\text{full})}, \boldsymbol{\beta}_{\text{PC}}^{(\text{ig})})$  versus the squared root of the squared Mahalanobis distance between the two classes,  $\Delta$ , for  $\pi_1 = 0.4$ .
